# Supplementary material for: Adaptive Weighted Total Variation boosted by learning techniques in few-view tomographic imaging
Source: arXiv:2501.09845 source file (2025-01-16)
Supplement: Supplementary file 1 [file 6_appendix_CP.tex]

\section{The Chambolle-Pock method for the solution of the proposed weighted-TV model}\label{sec:Appendix}
In its original formulation, the Chambolle-Pock method \cite{chambolle2011first}  was introduced to minimize an objective function of the form:
\begin{align}
    \min_{\x \in \R^n} F(\M\x) + G(\x),
\end{align}
where both $F$ and $G$ are real-valued, proper, convex, lower semi-continuous functions and $\M$ is a linear operator from $\R^n$ to $\R^s$. 
Note that there are no constraints on the smoothness of either $F$ and $G$; therefore, the method can be applied to our problem by setting:
\begin{align}
    \begin{cases}
        G(\x) = \iota_{\X}(\x), \\
        F(\M\x) = \mathcal{J}_{\Psi, \delta}(\x) = \frac{1}{2} || \K\x - \y^\delta ||_2^2 + \lambda || \w(\Psi(\y^\delta)) \odot | \D \x | ||_1,
    \end{cases}
\end{align}
where $\iota_{\X}(\x)$ is the indicator function of the feasible set $\X$. As already stated, we consider $\X$ as the non-negative subspace of $\R^n$.\\
To apply the CP method to our problem, we define the linear operator $\M \in \R^{s \times n}$  by concatenating row-wise $\K$ and $\D$, namely $\M = \left[ \K; \D \right]$ and $s=(m + 2n)$. The CP algorithm considers the primal-dual formulation of \eqref{eq:CP_general_formulation}, which reads:
\begin{align}
    \min_{\x \in \R^n} \max_{\z \in \R^{m+2n} } \z^T \M \x + G(\x) - F^*(\z),
\end{align}
where $F^*$ is the convex conjugate of $F$ \cite{bauschke2017correction}, defined as:
\begin{align}
    F^*(\z^*) := \sup_{\z \in \R^{m+2n} } \left\{ \z^T \z^* - F(\z) \right\}.
\end{align} 
Given a starting guess for both the primal variable $\x^{(0)}$ and the dual variable $\z^{(0)}$, the update rule is the following:
\begin{align}\label{eq:CP_iterates}
    \begin{cases}
        \z^{(k+1)} = \prox_{\sigma F^*}\left(\z^{(k)} + \sigma \M\bar{\x}^{(k)}\right), \\
        \x^{(k+1)} = \prox_{\tau G}\left(\x^{(k)} - \tau \M^T\z^{(k+1)}\right), \\
        \bar{\x}^{(k+1)} = \x^{(k+1)} + \beta \left(\x^{(k+1)} - \x^{(k)} \right),
    \end{cases}
\end{align}
where $\bar{\x}^{(0)} = \boldsymbol{0}$, $\beta \in [0, 1]$ is a parameter that we set equal to 1 in the experiments, while $\sigma > 0$, $\tau > 0$ are computed as $\sigma = \tau \approx \frac{1}{|| \boldsymbol{M} ||_2}$. A reliable approximation of $|| \boldsymbol{M} ||_2$ can be computed by means of the power iteration method  \cite{epperson2021introduction}. 

Focusing on $G(\x)$, its proximal operator corresponds to the projection $\mathcal{P}_+$ over the non-negative subspace $\X$. Consequently the updating rule of the primal variable $\x^{(k)}$ becomes:
\begin{align}
    \x^{(k+1)} = \mathcal{P}_+\left(\x^{(k)} - \tau \M^T\z^{(k+1)}\right).
\end{align}
The explicit derivation of $\prox_{\sigma F^*}$ requires the introduction of two dual variables, $\p \in \R^m$ and $\q \in \R^{2n}$, such that:
\begin{align}
    F(\p, \q) = \underbrace{\frac{1}{2} || \p - \y^\delta ||_2^2}_{:= F_1(\p)} + \underbrace{\lambda || \w(\tilde{\x}) \odot | \q | ||_1}_{:= F_2(\q)}.
\end{align}
Denominating $F_1(\p) = \frac{1}{2} || \p - \y^\delta ||_2^2$, its convex conjugate $F_1^*(\p)$ can be easily computed as:
\begin{align}
    F_1^*(\p) &= \sup_{\p'} \left\{ \p^T \p' - \frac{1}{2} || \p' - \y^\delta ||_2^2 \right\} \\ &= \p^T \y^\delta + \frac{3}{2} || \p ||_2^2,
\end{align}
\AS{
Il gradiente dovrebbe essere 
\begin{equation*}
    \p-(\p'-\y^\delta)=0\Rightarrow \p' =\p + \y^\delta
\end{equation*}
Quindi se vado a sostituire (A.9)
\begin{equation*}
    F_1^*(\p) = \|\p\|_2^2+\p^T\y^\delta - \frac{1}{2}\|\p\|_2^2 = \p^T\y^\delta + \frac{1}{2}\|\p\|_2^2
\end{equation*}
}
since the problem defining $F_1^*$ is quadratic in $\p'$ and it can be solved by imposing the optimality condition of null gradient. %computing its gradient and setting it to zero.
Consequently, the proximal map of $F_1^*$ gets:
\begin{align}
    \prox_{\sigma F_1^*}(\p) &= \arg\min_{\p'} (\p')^T \y^\delta + \frac{3}{2} || \p' ||_2^2 + \frac{1}{2\sigma} || \p' - \p ||_2^2 \\&= \frac{\p - \sigma \y^\delta}{1 + 3\sigma}.
\end{align}
\AS{
Questo invece dovrebbe essere
\begin{align}
    \prox_{\sigma F_1^*}(\p) &= \arg\min_{\p'} (\p')^T \y^\delta + \frac{3}{2} || \p' ||_2^2 + \frac{1}{2\sigma} || \p' - \p ||_2^2 \\&= \frac{\p - \sigma \y^\delta}{1 + \sigma}.
\end{align}
quindi andrebbe cambiato anche in sotto.
}
Similarly, calling $F_2(\q) = \lambda || \w(\tilde{\x}) \odot | \q | ||_1$, we derive:
\begin{align}
    F_2^*(\q) = \begin{cases}
        0 \quad &\text{if } \q \leq \lambda \w(\tilde{\x}), \\
        \infty \quad &\text{otherwise}, 
    \end{cases}
\end{align}
which implies that:
\begin{align}
\begin{split}
    \prox_{\sigma F_2^*}(\q) &= \arg\min_{\q'} F_2^*(\q') + \frac{1}{2\sigma} || \q - \q' ||_2^2 = \frac{\lambda \w(\tilde{\x}) \odot \q}{\max \left( \lambda \w(\tilde{\x}), \q \right)},
\end{split}
\end{align}
where both the maximum and the division are taken element-wise. More details on the computation of the proximal operator of $F_2^*$ can be found in \cite{sidky2014cttpv}. \\

Plugging these results into the CP scheme \eqref{eq:CP_iterates} with $\z^{(k)} = (\p^{(k)}, \q^{(k)})$, leads to the following updating rules:
\begin{align}
    \begin{cases}
        \p^{(k+1)} = \frac{\p^{(k)} + \sigma \left(\K \bar{\x}^{(k)} - \y^\delta \right)}{1 + 3\sigma}, \\
        \q^{(k+1)} = \frac{\lambda \w(\tilde{\x}) \odot \left(\q^{(k)} + \sigma | \D \bar{\x}^{(k)} | \right)}{\max \left( \lambda \w(\tilde{\x}), \q^{(k)} + \sigma | \D \bar{\x}^{(k)} | \right)}, \\
        \x^{(k+1)} = \mathcal{P}_+\left(\x^{(k)} - \tau \M^T\begin{bmatrix}
            \p^{(k+1)} \\ \q^{(k+1)}
        \end{bmatrix} \right), \\
        \bar{\x}^{(k+1)} = \x^{(k+1)} + \beta \left(\x^{(k+1)} - \x^{(k)} \right).
    \end{cases}
\end{align}
The corresponding CP algorithm is reported in Algorithm \ref{algo1}. 
We remark that the CP algorithm is convergent if both $F(\M\x)$ and $G(\x)$ are convex, proper and lower semi-continuous, with a theoretical convergence rate of $\mathcal{O}(\frac{1}{k^2})$ \cite{chambolle2011first}, and we fit these requirements.

\AS{In realtà servono che $F^*$ e $G$ siano uniformly convex, e lo dimostrano scegliend una sequenza di $\beta$ crescente.}

\begin{algorithm}
\caption{The Chambolle-Pock algorithm to solve Problem \eqref{eq:Psi_Wl1_formulation}}\label{algo1}
\begin{algorithmic}[1]
\Require a linear operator $\K$, corrupted data $\y^\delta \in \R^m$, a regularization parameter $\lambda > 0$, an initial guess $\tilde{\x} \in \R^n$
\Require $\bar{\x}^{0} = \x^{0} \in \R^n$, $\p^{(0)} \in \R^m$, $\q^{(0)} \in \R^{2n}$
\State \textbf{define} $\M = \left[ \K; \D \right]$, $\gamma \approx || \M ||_2, \tau = \sigma = \gamma^{-1}$, $\beta = 1$, $\eta > 0$
\State \textbf{initialize} $k = 0$
\Repeat
    \State $\p^{(k+1)} = \frac{\p^{(k)} + \sigma \left(\K \bar{\x}^{(k)} - \y^\delta \right)}{1 + 3\sigma}$ \Comment{Update dual variables}
    \State $\q^{(k+1)} = \frac{\lambda \w(\tilde{\x}) \odot \left(\q^{(k)} + \sigma | \D \bar{\x}^{(k)} | \right)}{\max \left( \lambda \w(\tilde{\x}), \q^{(k)} + \sigma | \D \bar{\x}^{(k)} | \right)}$
    \State
    \State $\x^{(k+1)} = \mathcal{P}_+\left(\x^{(k)} - \tau \M^T\begin{bmatrix}
            \p^{(k+1)} \\ \q^{(k+1)}
        \end{bmatrix} \right)$ \Comment{Update primal variable}
    \State
    \State $\bar{\x}^{(k+1)}=\x^{(k+1)}+\beta(\x^{(k+1)}-\x^{(k)})$ \Comment{Update inertia term}
    \State
    \State \textbf{update } $k = k + 1$
\Until{convergence}
\end{algorithmic}
\end{algorithm}
